# Supplementary material for: Classification of Legendrian knots of topological type $7_6$ with maximal Thurston--Bennequin number
Source: arXiv:1901.03600 ancillary file (2019-01-11)
Supplement: Supplementary file 1 [file realizations-r7.pdf]

The diagram  $R_7$

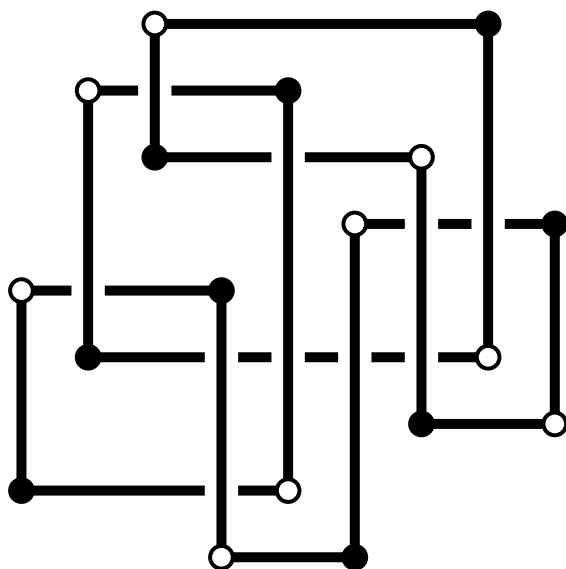

Sequence code:

$[3, 3, -4, 2, 5, 3, -3, -2, 4, -4, 2, 5, -5, -6, 4, 3, -6, -4].$

#1: Realization of  $(\delta_2^+, \delta_2^-)$

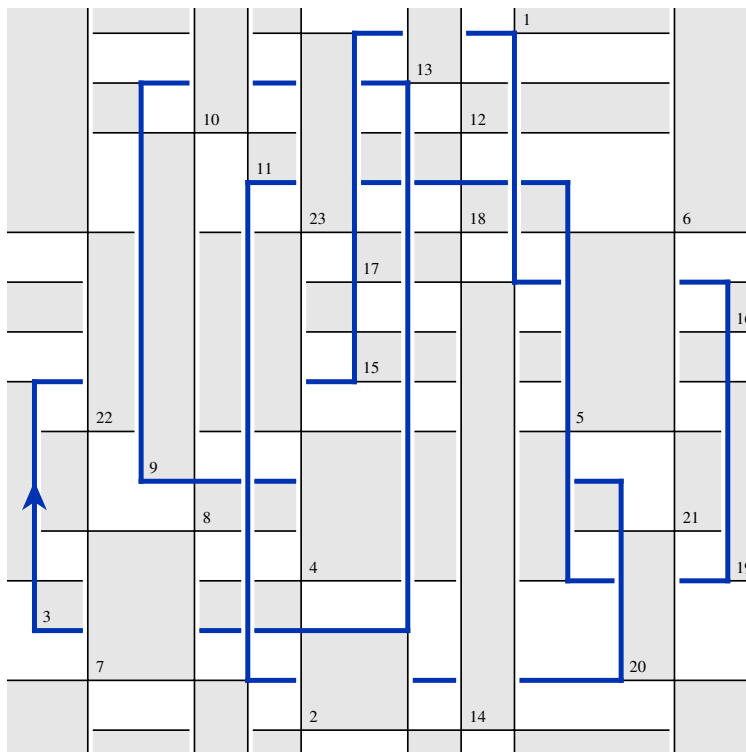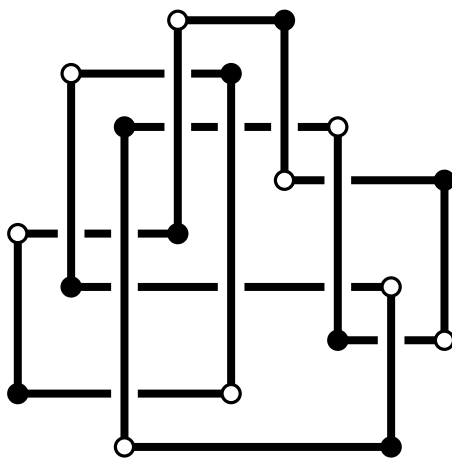

Sequence code:

$$[3, 3, 4, 2, -3, 3, -3, -2, 4, -4, -6, 5, 3, -6, 4, 3, -6, -4]$$

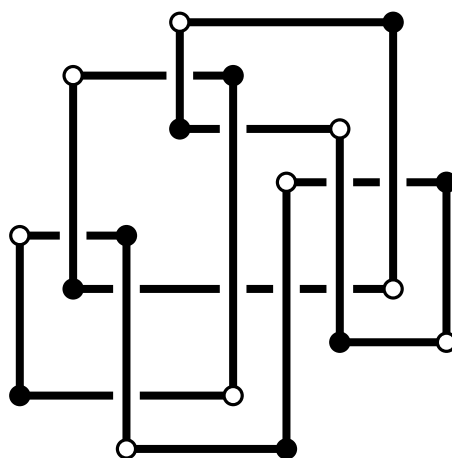
$$[3, 2, -4, 3, 5, 3, -3, -2, 4, -3, 2, 4, -5, -6, 4, 3, -6, -4]$$

#3: Realization of  $(\delta_2^+, \delta_2^-)$   
 (this is the diagram from Figure 7)

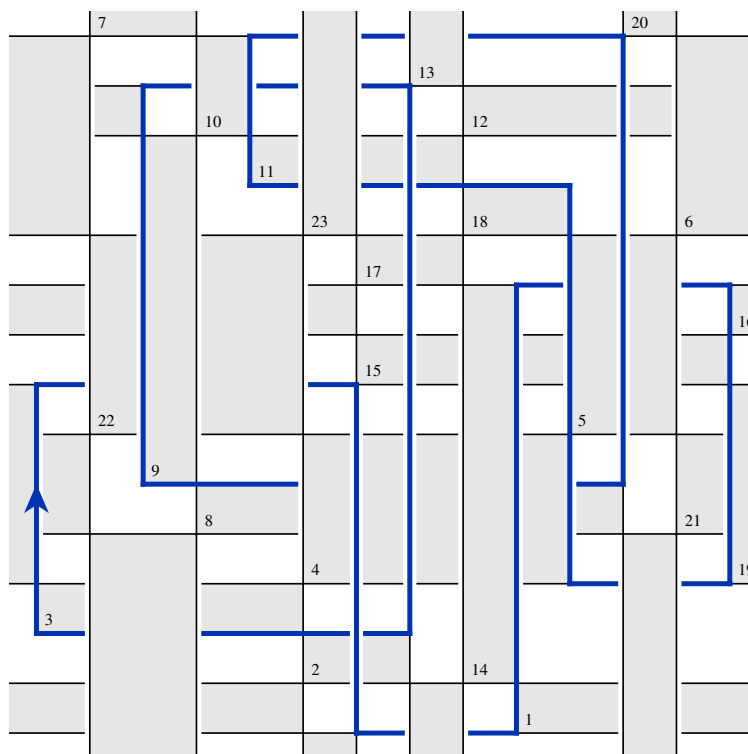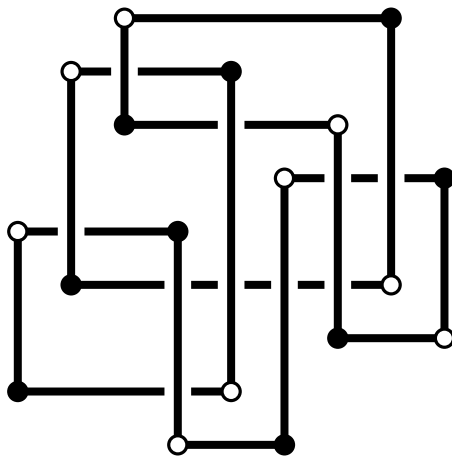

Sequence code:

$[3, 3, -4, 2, 5, 3, -3, -2, 4, -4, 2, 5, -5, -6, 4, 3, -6, -4]$ .

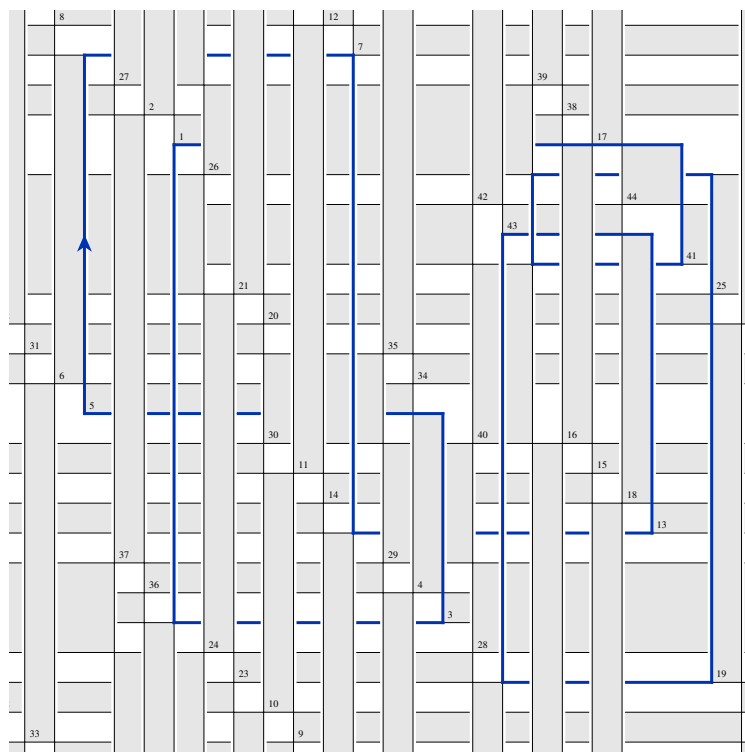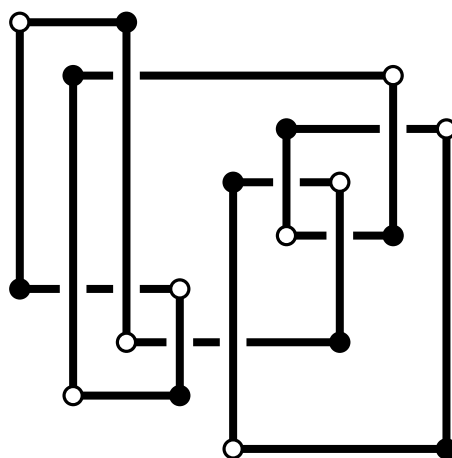

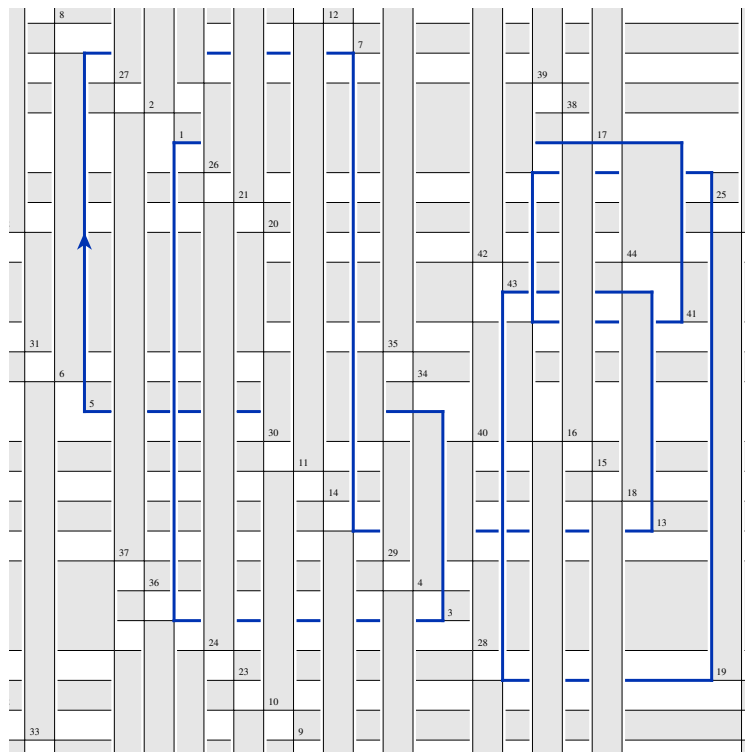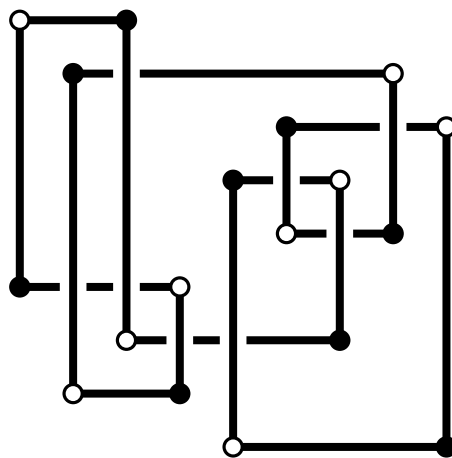

#6: Realization of  $(\delta_2^+, \sigma(\delta_2^-))$

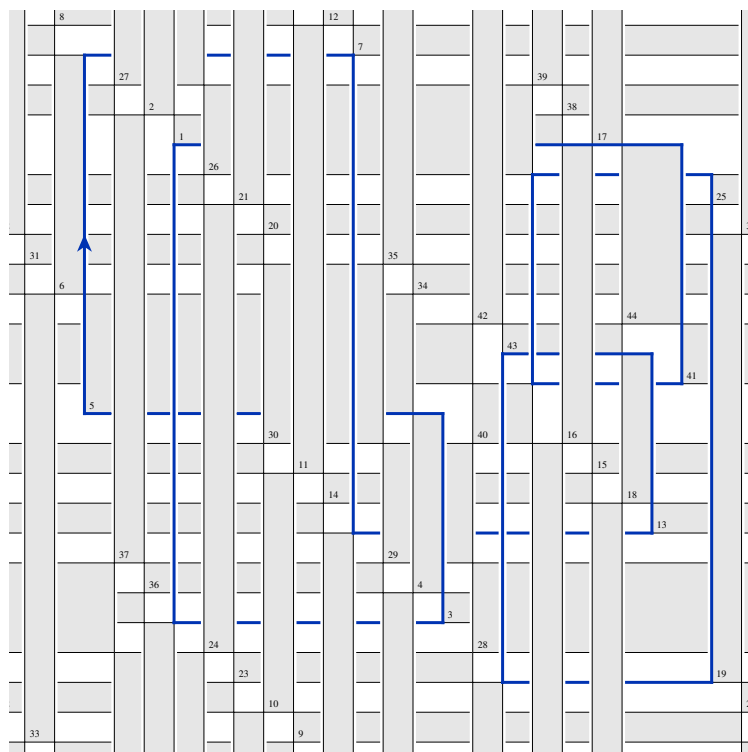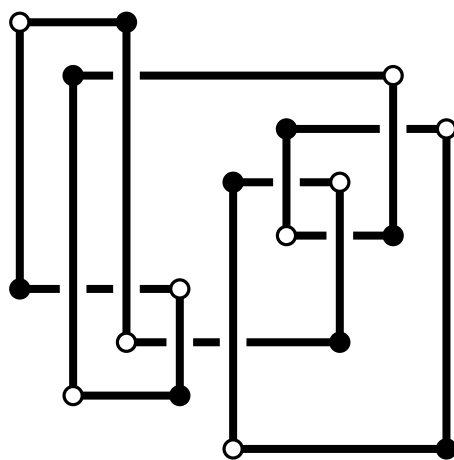

#7: Realization of  $(\delta_2^+, \sigma(\delta_2^-))$

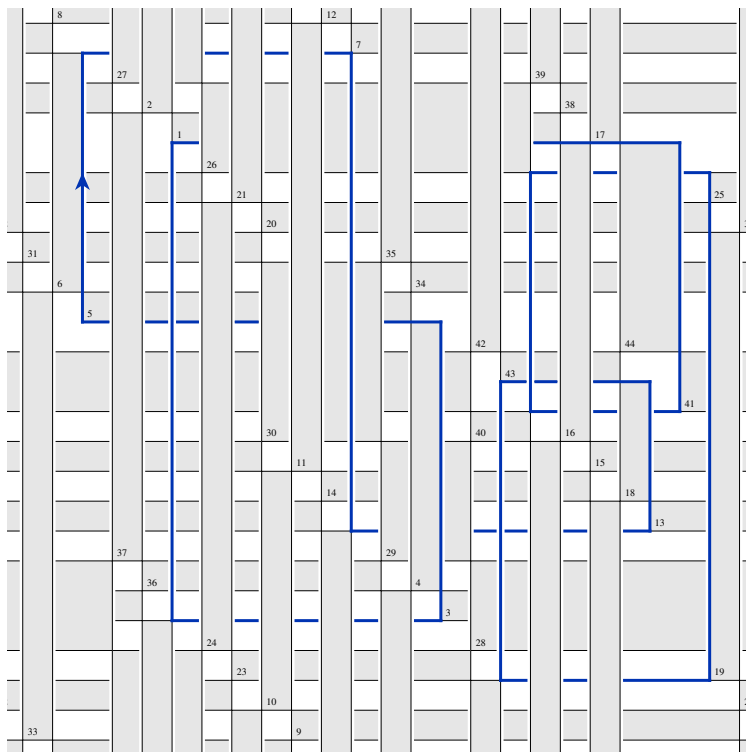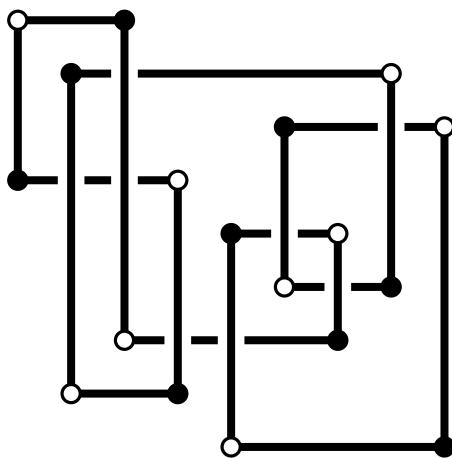



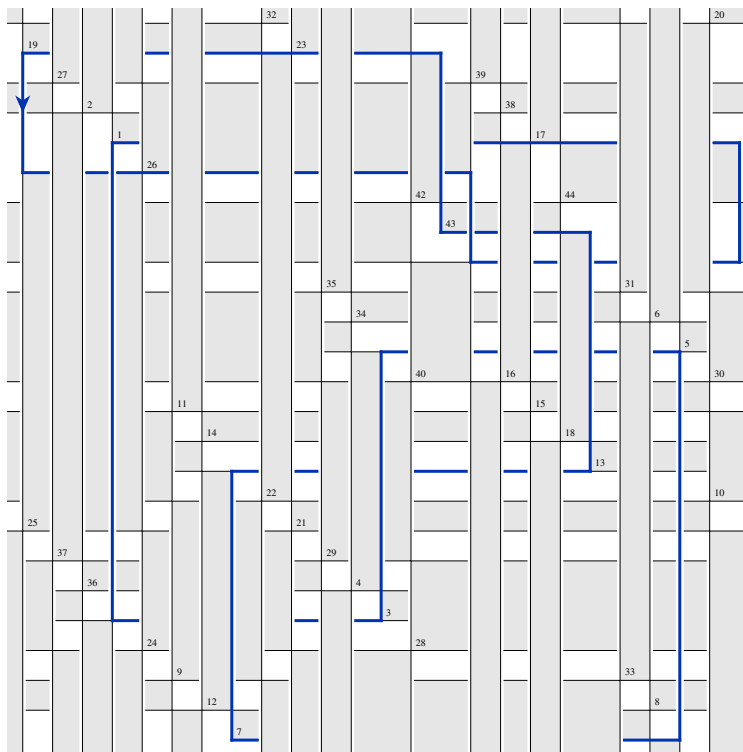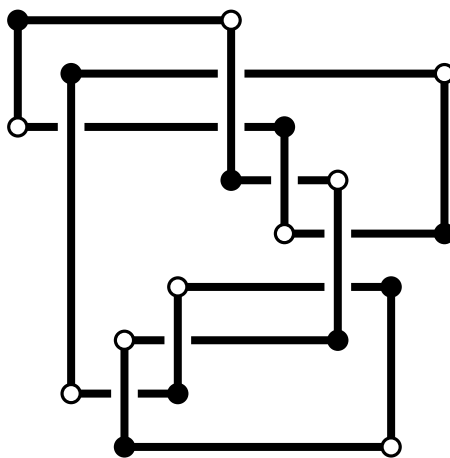

#9: Realization of  $(\delta_2^+, \sigma(\delta_2^-))$

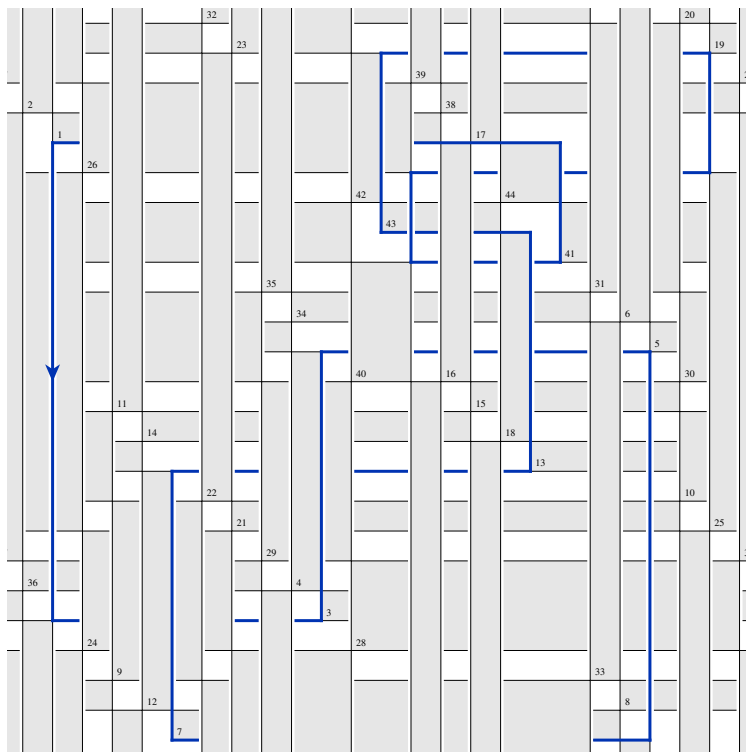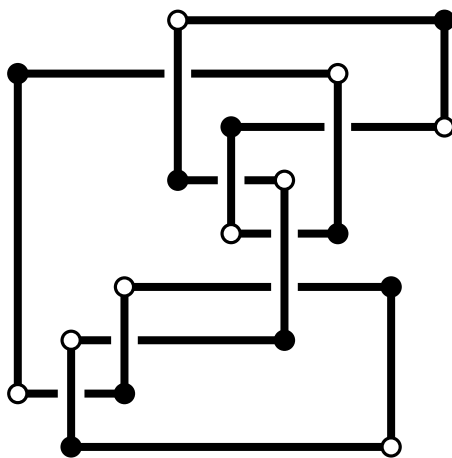

#10: Realization of  $(\delta_2^+, \sigma(\delta_2^-))$

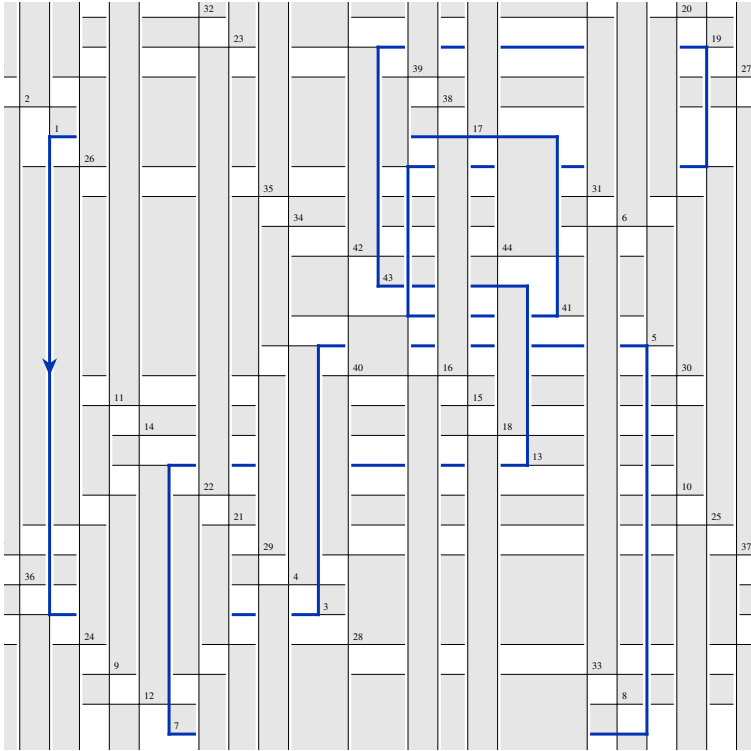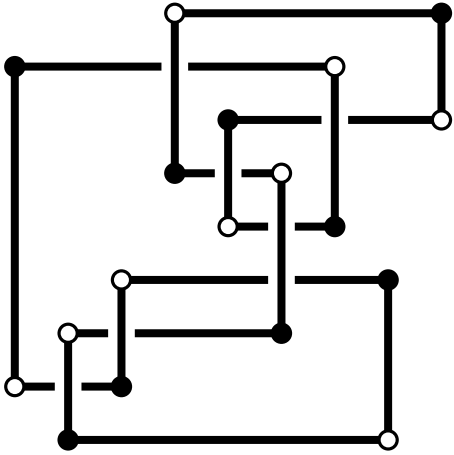

#11: Realization of  $(\delta_2^+, \sigma(\delta_2^-))$

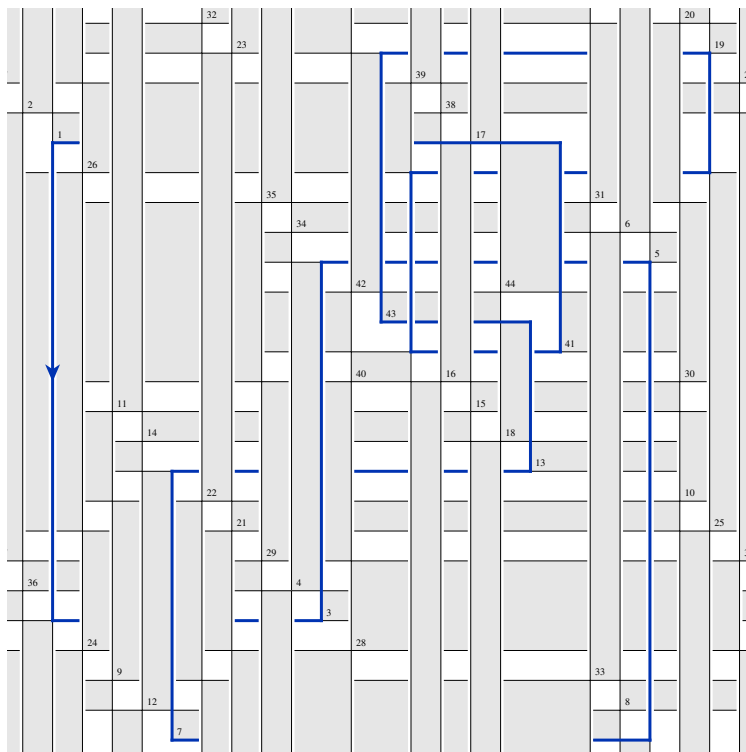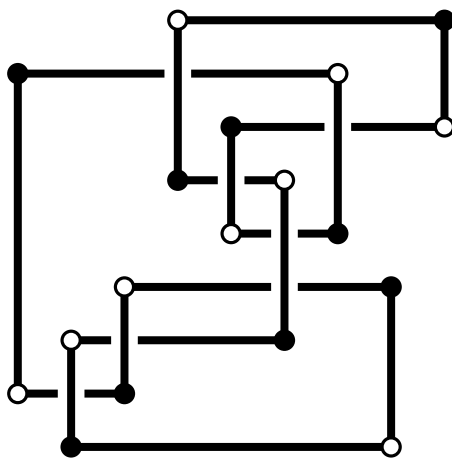

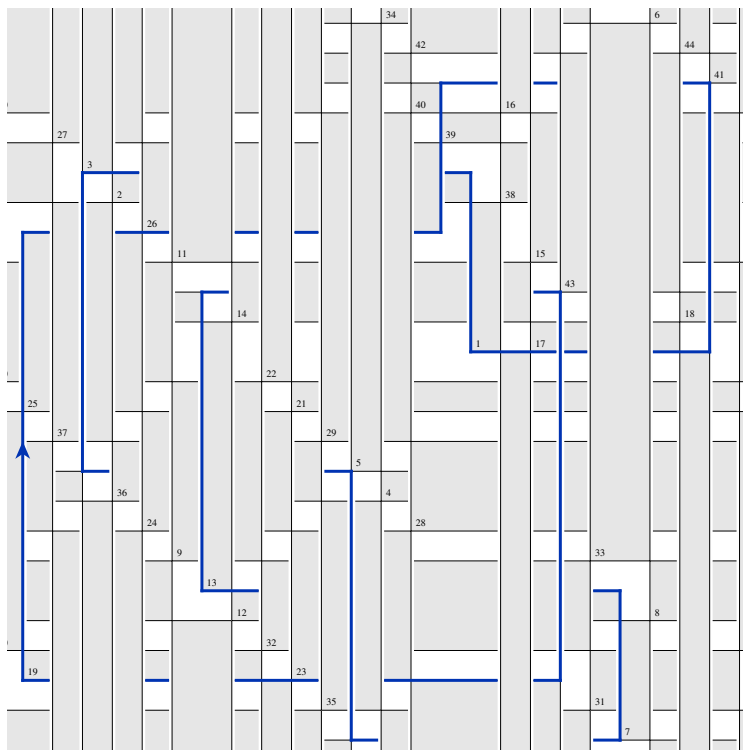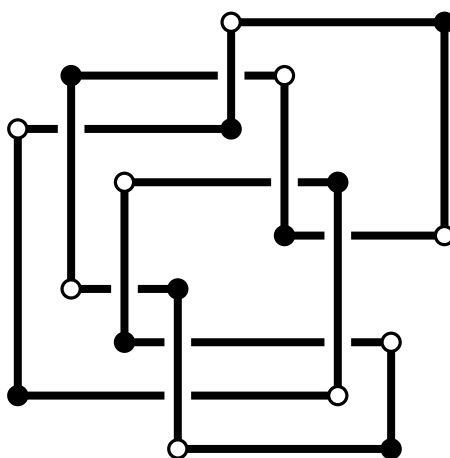
$$[5, 4, 2, 4, -4, -3, 3, -4, -4, 2, -3, 4, 2, -5, 3, 4, -4, -6]$$

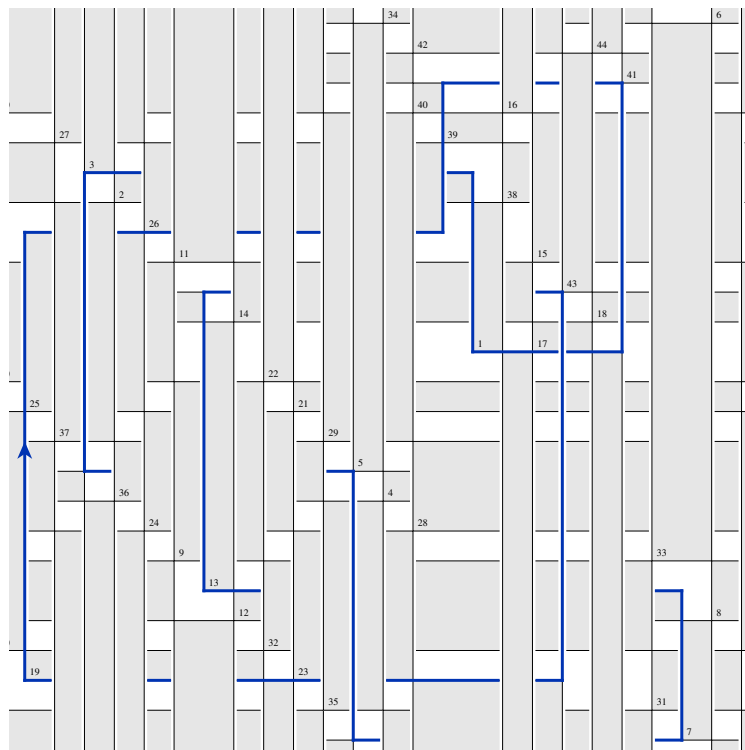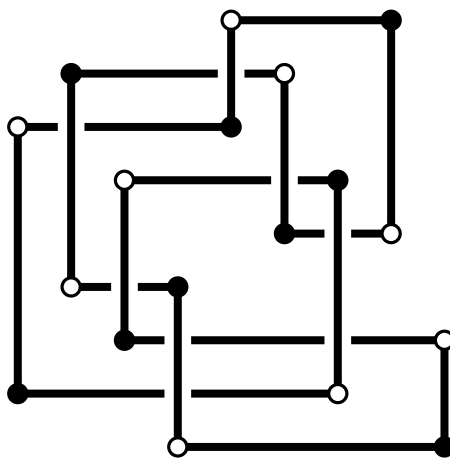
$$[5, 4, 2, 3, -4, -2, 3, -4, -4, 2, -3, 5, 2, -6, 3, 4, -4, -6]$$

#14: Realization of  $(\delta_2^+, \sigma(\delta_2^-))$

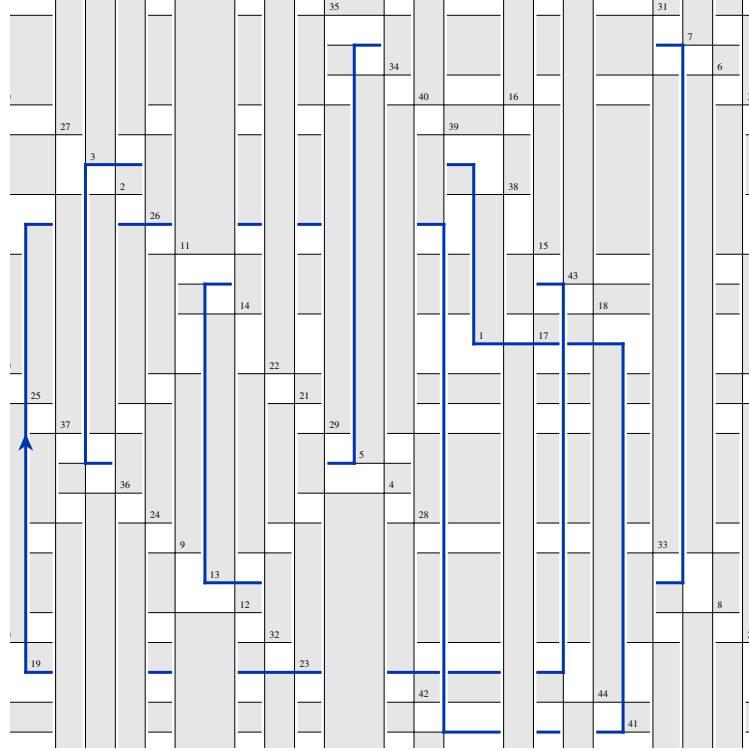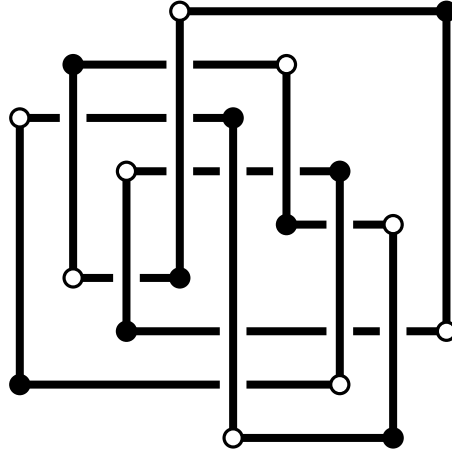

Sequence code:

$[5, 4, -6, 3, 4, -2, 3, -4, -4, 2, 5, 5, -6, -6, 3, 4, -4, -6]$

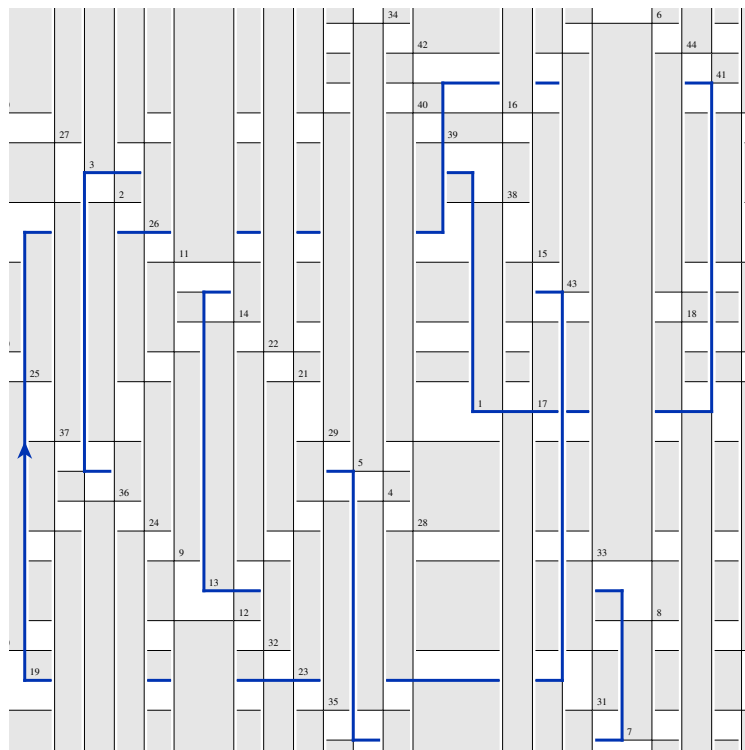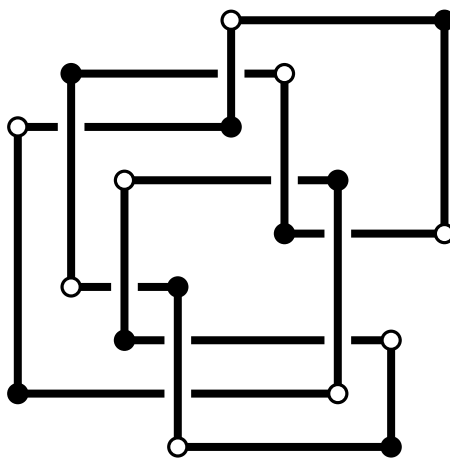
$$[5, 4, 2, 4, -4, -3, 3, -4, -4, 2, -3, 4, 2, -5, 3, 4, -4, -6]$$



#16: Realization of  $(\delta_2^+, \sigma(\delta_2^-))$

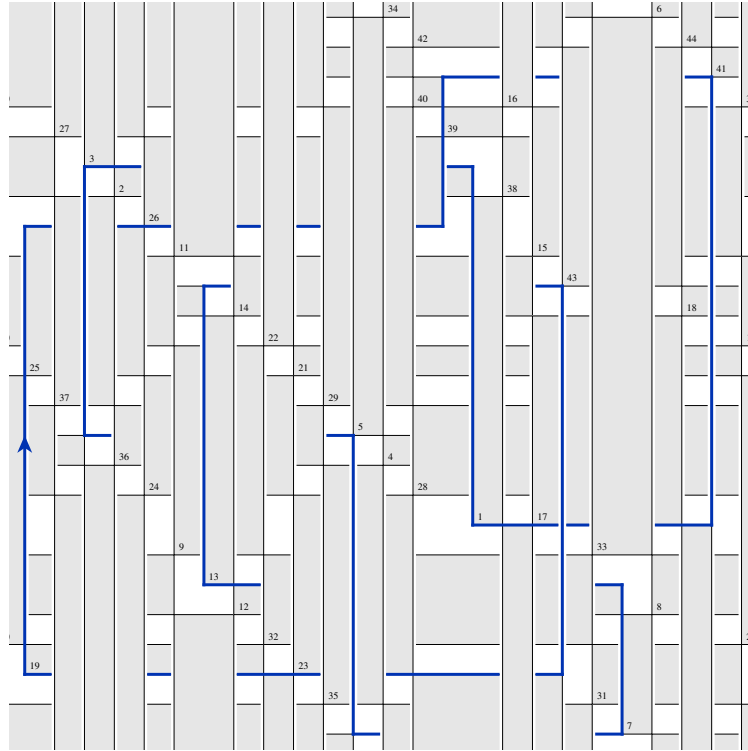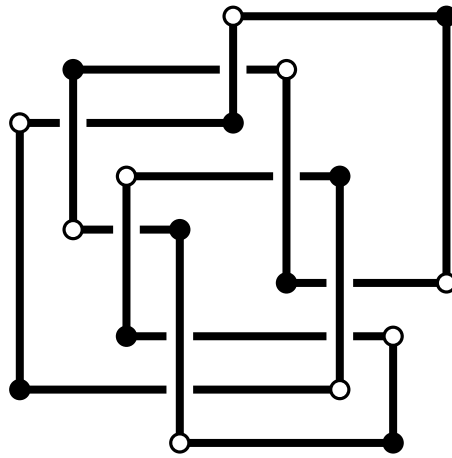

Sequence code:

$[5, 4, 2, 4, -5, -3, 4, -4, -3, 2, -4, 4, 2, -5, 3, 4, -4, -6]$

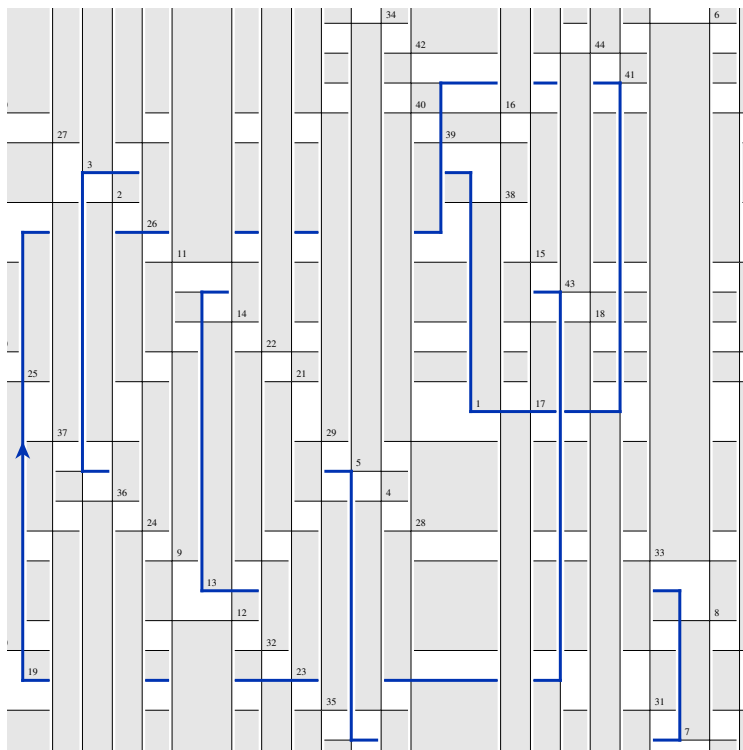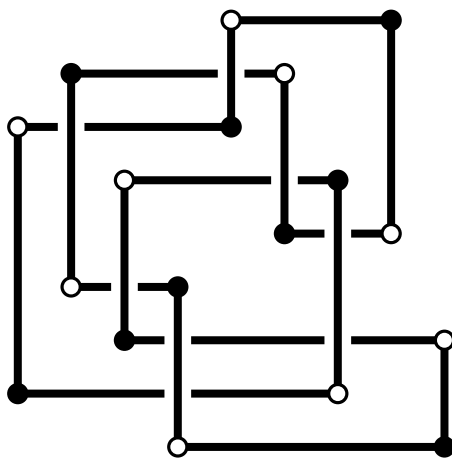
$$[5, 4, 2, 3, -4, -2, 3, -4, -4, 2, -3, 5, 2, -6, 3, 4, -4, -6]$$

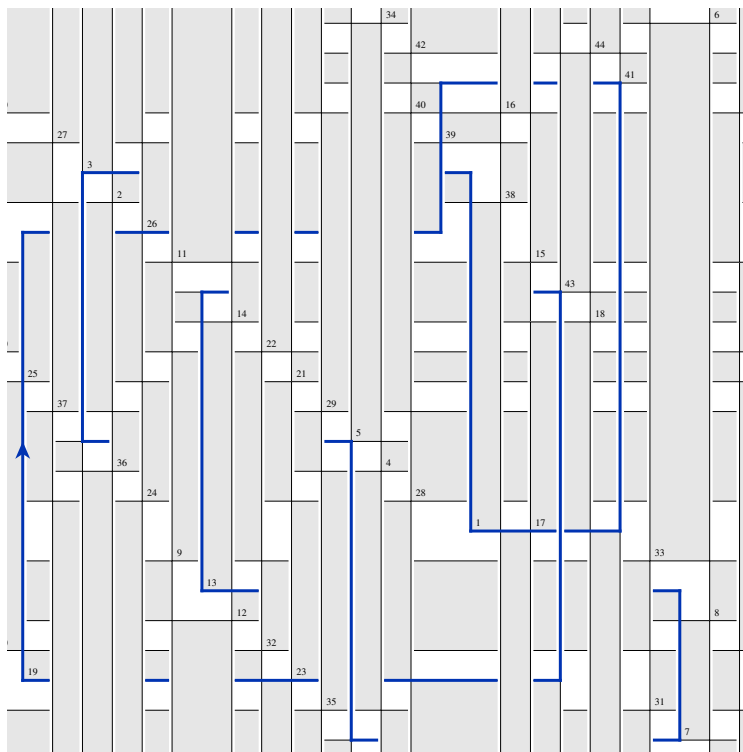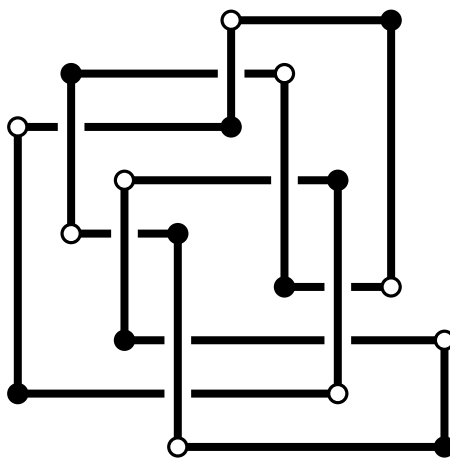
$$[5, 4, 2, 3, -5, -2, 4, -4, -3, 2, -4, 5, 2, -6, 3, 4, -4, -6]$$

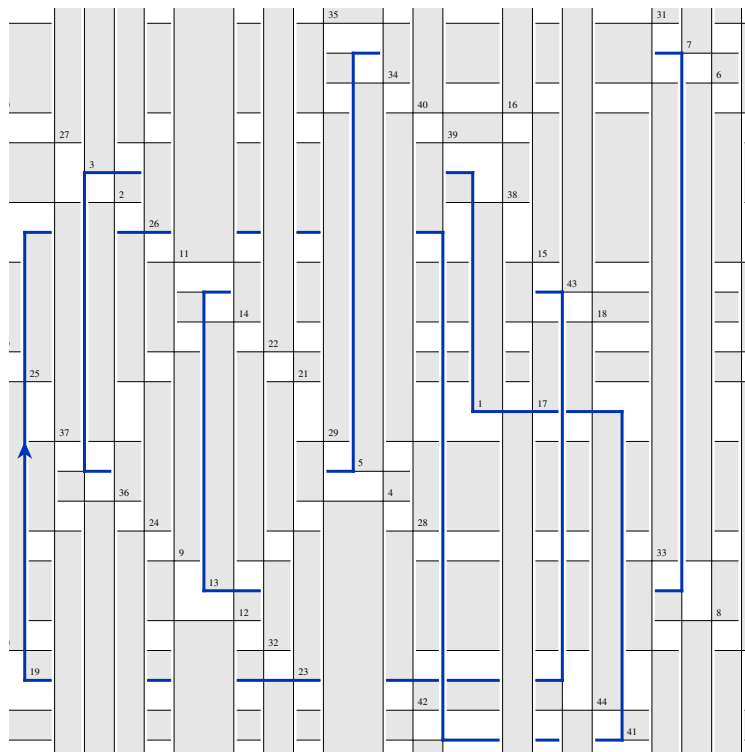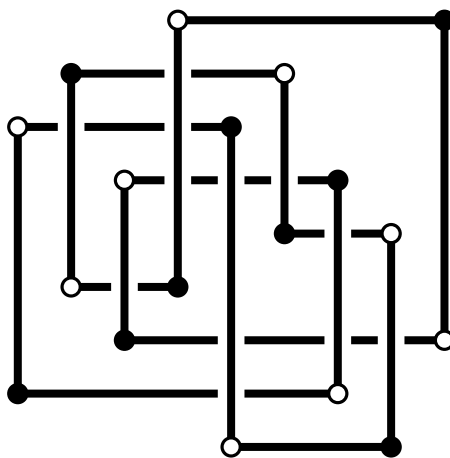
$$[5, 4, -6, 3, 4, -2, 3, -4, -4, 2, 5, 5, -6, -6, 3, 4, -4, -6]$$

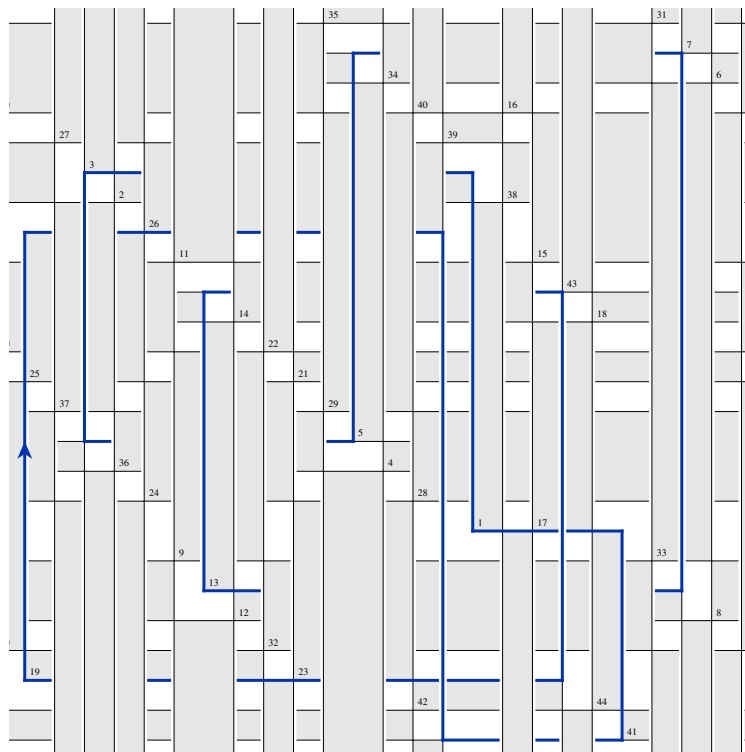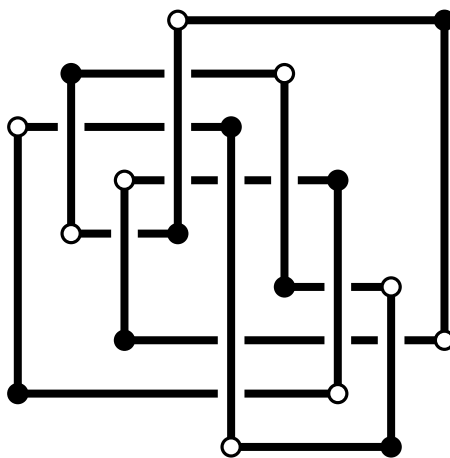
$$[5, 4, -6, 3, 3, -2, 4, -4, -3, 2, 4, 5, -6, -6, 3, 4, -4, -6]$$

#21: Realization of  $(\delta_2^+, \sigma(\delta_2^-))$

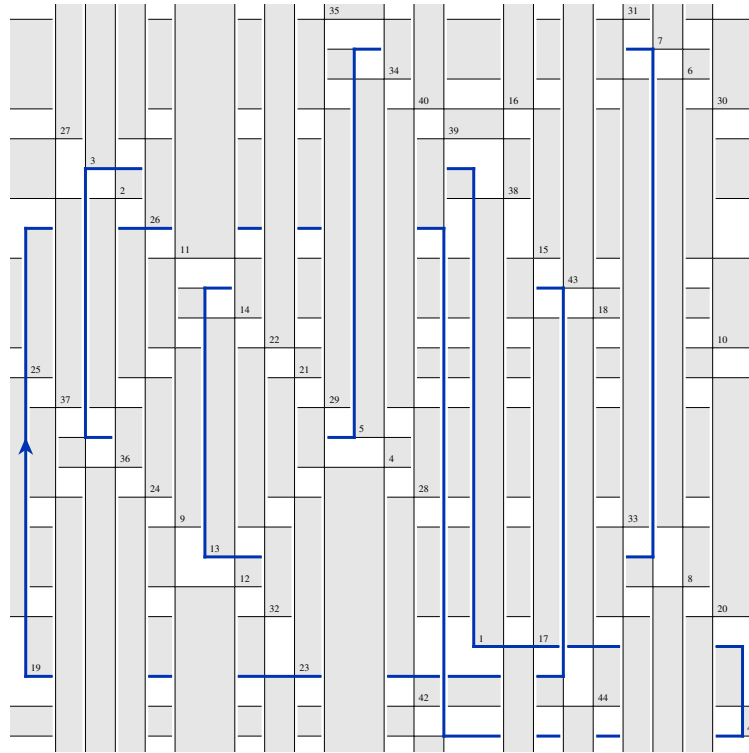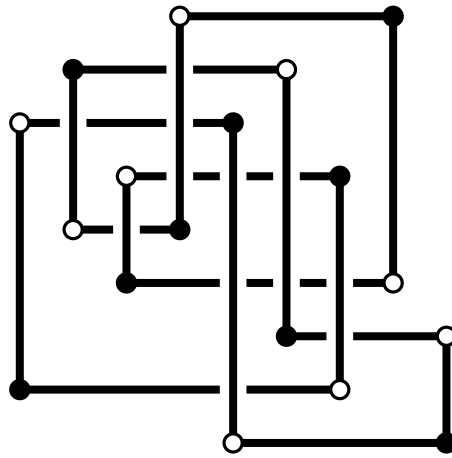

Sequence code:

$[5, 4, -6, 4, 2, -3, 5, -4, -3, 2, 4, 4, -5, -5, 2, 4, -4, -6]$

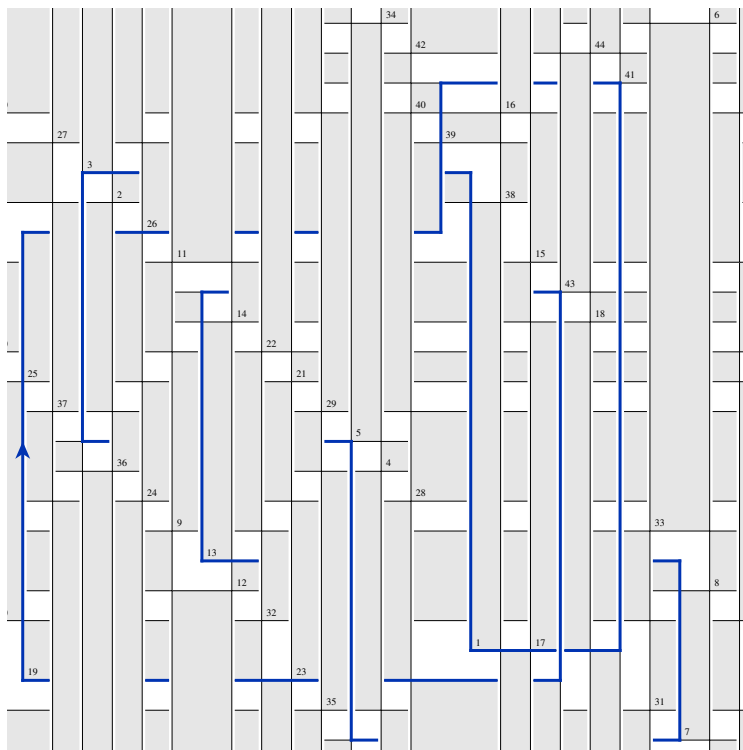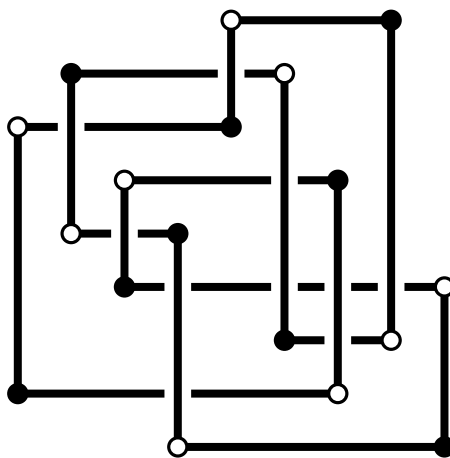
$$[5, 4, 2, 3, -6, -2, 5, -4, -3, 2, -4, 5, 3, -6, 2, 4, -4, -6]$$

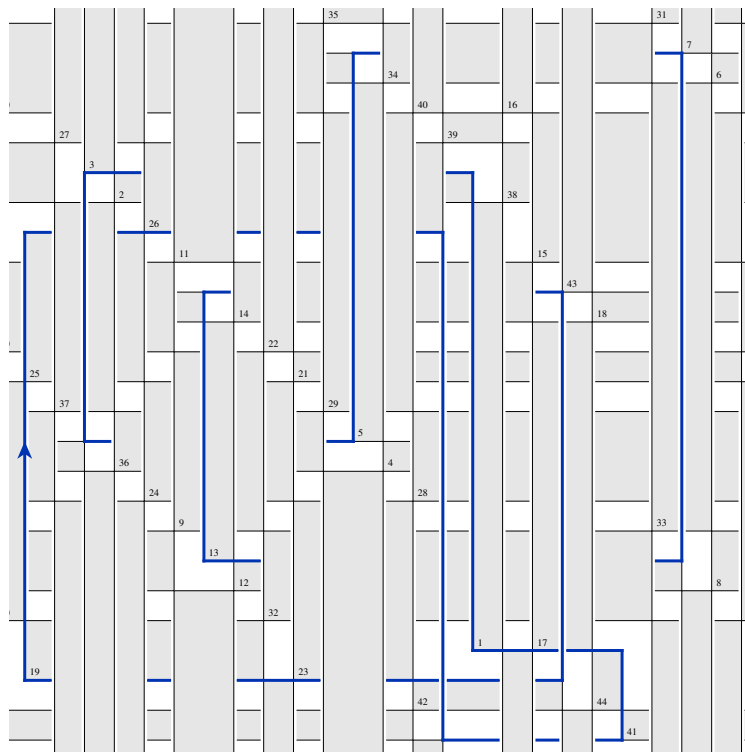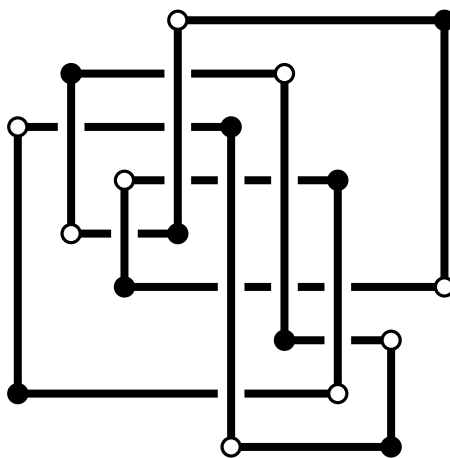
$$[5, 4, -6, 3, 2, -2, 5, -4, -3, 2, 4, 5, -5, -6, 2, 4, -4, -6]$$
